# Supplementary material for: Automated Long Answer Grading with RiceChem Dataset
Source: arXiv:2404.14316 source file (2024-04-22)
Supplement: Supplementary file 1 [file appendix_baselines_table.tex]

% \begin{table*}[h!]
% \centering
% \normalsize
% \begin{tabular}{lllll}
%   \hline
%   \textbf{Model} & \textbf{Accuracy} & \textbf{Precision} & \textbf{Recall} & \textbf{F1} \\
%   \hline
%   BERT-large & 0.015 & 0.020 & 0.036 & 0.021 \\
%   BERT-large-mnli & 0.019 & 0.019 & 0.033 & 0.025\\
%   RoBERTa-large & 0.010 & 0.025 & 0.012 & 0.009\\
%   RoBERTa-large-mnli & 0.011 & 0.012 & 0.035 & 0.016\\
%   BART-large & 0.008 & 0.012 & 0.008 & 0.009\\
%   BART-large-mnli & 0.007 & 0.018 & 0.018 & 0.008\\
%   GPT3.5 & N/A & N/A & N/A & N/A\\
%   GPT4 & N/A & N/A & N/A & N/A\\
%   \hline
% \end{tabular}
% \caption{\label{tab:results}Standard deviations of baselines.}
% \end{table*}
