# Supplementary material for: Automated Long Answer Grading with RiceChem Dataset
Source: arXiv:2404.14316 source file (2024-04-22)
Supplement: Supplementary file 2 [file appendix_comparisons.tex]

% \begin{figure*}
%   \centering
%   \begin{subfigure}[b]{0.49\textwidth}
%     \includegraphics[width=\textwidth]{emnlp2023-latex/figures/accuracy_comparison.pdf}
%     \caption{Comparison: accuracy}
%     \label{fig:accuracy_comparison}
%   \end{subfigure}
%   \hfill
%   \begin{subfigure}[b]{0.49\textwidth}
%     \includegraphics[width=\textwidth]{emnlp2023-latex/figures/precision_comparison.pdf}
%     \caption{Comparison: precision}
%     \label{fig:precision_comparison}
%   \end{subfigure}

%   \vspace{0cm} % Adjust the vertical spacing between the top and bottom subfigures

%   \begin{subfigure}[b]{0.49\textwidth}
%     \includegraphics[width=\textwidth]{emnlp2023-latex/figures/recall_comparison.pdf}
%     \caption{Comparison: recall}
%     \label{fig:recall_comparison}
%   \end{subfigure}
%   \hfill
%   \begin{subfigure}[b]{0.49\textwidth}
%     \includegraphics[width=\textwidth]{emnlp2023-latex/figures/f1_comparison.pdf}
%     \caption{Comparison: f1}
%     \label{fig:f1_comparison}
%   \end{subfigure}

%   \vspace{0cm} % Adjust the vertical spacing between the top and bottom subfigures

%   \begin{subfigure}[b]{0.49\textwidth}
%     \includegraphics[width=\textwidth]{emnlp2023-latex/figures/mse_comparison.pdf}
%     \caption{Comparison: MSE}
%     \label{fig:mse_comparison}
%   \end{subfigure}
%   \hfill
%   \begin{subfigure}[b]{0.49\textwidth}
%     \includegraphics[width=\textwidth]{emnlp2023-latex/figures/mae_comparison.pdf}
%     \caption{Comparison: MAE}
%     \label{fig:mae_comparison}
%   \end{subfigure}

%   \caption{Comparisons of performance using \model and the traditional ASAG. We achieve significant improvements after applying \model on both discriminative and generative models.}
%   \label{fig:baseline}
% \end{figure*}
